# Supplementary material for: High-harmonic generation in solids with and without topological edge states
Source: arXiv:1711.05783 ancillary file (2018-01-31)
Supplement: Supplementary file 1 [file supplmat_topologicalhhg.pdf]

# Supplemental Material: High-harmonic generation in solids with and without topological edge states


Dieter Bauer
*Institute of Physics, University of Rostock, 18051 Rostock, Germany*

Kenneth K. Hansen
*Department of Physics and Astronomy, Aarhus University, DK-8000, Denmark*



(Dated: January 26, 2018)


## I. ODD NUMBER OF IONS

With an odd number of singly charged ions and one electron per ion, the Kohn-Sham (KS) system is necessarily spin-polarized. Phase A and B become equivalent in this case, apart from the fact that in phase A there remains one undimerized atom at the right edge and in phase B at the left edge. Figure 1 shows the band structure for phase A with $a = 2$, $N = 101$, $N_\uparrow = 51$, $N_\downarrow = 50$, $\delta = 0.265$. The undimerized atom at the right edge leads to an edge state in the spin-up band structure that is located *below* the valence band. In fact, the KS orbital of lowest energy is spatially localized at the right edge. The lowest KS orbital of the spin-down electrons compensates this and has more probability density in the left half of the chain. The valence bands for both spin up and spin down are fully populated (plus the single, extra edge state below the valence band for spin up). As a consequence, destructive interference in the total dipole response is very pronounced, as can be seen in Fig. 2. Again, there are almost no sub-band-gap harmonics, as for phase A with an even number of ions. Hence, the mere presence of an edge state is not enough to generate harmonics in the sub-band-gap regime.

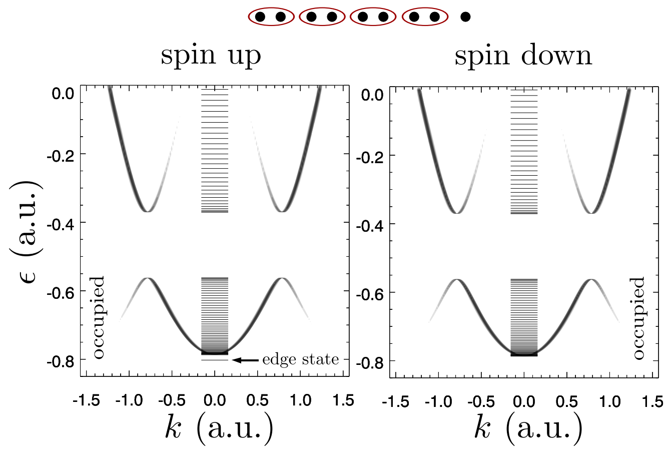


Figure 1. Band structures for the spin-up and spin-down KS electrons for $N = 101$ ions, $N_\uparrow = 51$, $N_\downarrow = 50$ electrons, (initial) lattice constant $a = 2$, and $\delta = 0.265$ (phase A). There is one undimerized ion at the right edge.

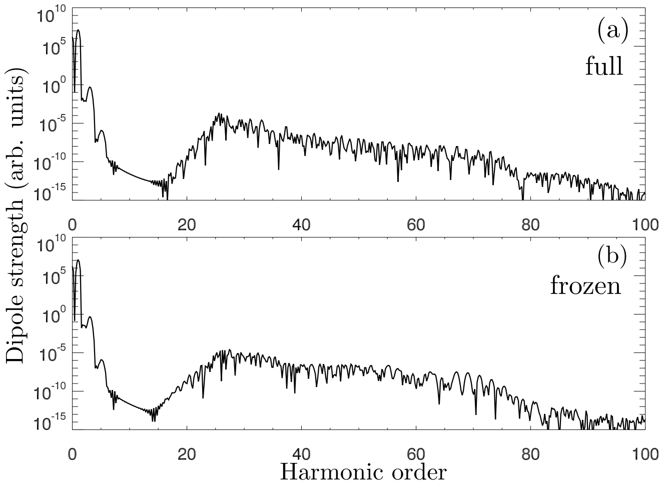


Figure 2. Harmonics emitted by the chain with $N = 101$ ions, $N_\uparrow = 51$, $N_\downarrow = 50$. The laser parameters are the same as in the Letter, i.e., $n_{\text{cyc}} = 5$-cycle $\sin^2$-shaped laser pulse of frequency $\omega = 0.0075$ (i.e., $\lambda \simeq 6.1\,\mu$m), $A_0 = 0.1$, corresponding to $\simeq 2 \times 10^{10}$ W/cm$^2$. The difference between the full TDDFT calculation (a) and the one with a frozen KS potential (b) is minor.

## II. PHASE A WITH IMPURITIES AT EDGES

Edge states in the band gap can be generated for phase A by impurity ions at the left and at the right boundary. We model the impurity ions by the choice of a different smoothing parameter $\varepsilon = 3$ in the soft-core Coulomb potential, i.e.,

$$v_{\text{impurity}}(x) = -\frac{1}{\sqrt{(x - x_i)^2 + \varepsilon}} \tag{1}$$

with $i = 1$ or $N$. For the other ions we keep $\varepsilon = 1$. The left panel in Fig. 3 shows the band structure for the spin-neutral case with $N = 100$, $N_\uparrow = N_\downarrow = N/2$, $a = 2$, $\delta = 0.265$. An isolated impurity atom with $\varepsilon > 1$ has a lower ionization potential than an isolated bulk atom with $\varepsilon = 1$. As a consequence, the highest *two* occupied KS orbitals are spatially localized at the edges, as seen in the right panel of Fig. 3. That is the main difference between phase A with such impurities and phase B: the topological phase B has two (almost) degenerate edge states in the band gap but only the lower (odd) one is populated. The two edge states in phase B thus form a half-filled "mini band" while phase A with impurities has a similar mini band which, however, is fully occupied. This difference

has pronounced consequences for harmonic generation, as is shown in Fig. 4.

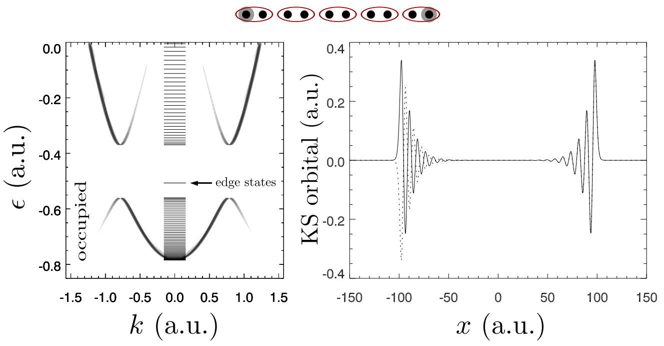


Figure 3. Left: Band structures for the spin-neutral phase A with $N = 100$, $N_\uparrow = N_\downarrow = N/2$, $a = 2$, $\delta = 0.265$ but with impurity ions with smoothing parameter $\varepsilon = 3$ at the left and the right boundary, leading to edge states within the band gap. Right: KS orbitals of the two almost degenerate edge states (lower, occupied, even orbital $\varphi_{49}(x)$ drawn solid; higher, occupied, odd orbital $\varphi_{50}(x)$ drawn dashed). Both are populated in the ground state configuration.

Despite the presence of edge states in the gap there are almost no sub-band-gap harmonics. The yield is higher than for the pure phase-A spectrum in Fig. 2 of the Letter but still far below phase B. The filled mini band in the phase-A impurity case leads to destructive interference, the half-filled mini band resulting from the topological edge states of phase B not.

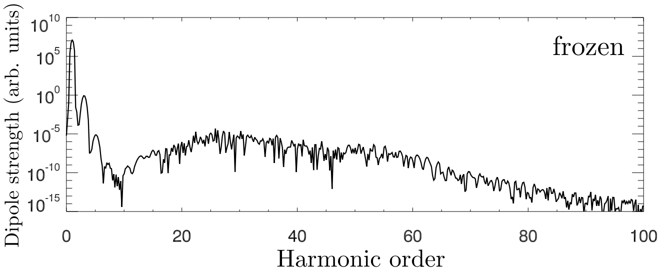


Figure 4. Harmonics emitted by the phase-A chain with $N = 100$ ions, $N_\uparrow = 50$, $N_\downarrow = 50$ and impurity ions at the left and right end. The laser parameters are the same as in the Letter. The result for the frozen KS potential is shown (the result for the full KS potential is very similar, as in all the other examples in this work).

## III. PHASE B WITH IMPURITIES AT EDGES

Adding the same kind of impurity to phase B shifts the already existing edge states in energy. With an increased smoothing parameter they shift to higher energy, as it is seen in Fig. 5 (compare to Fig. 1d in the Letter). The population of these states remains the same. The lower of the two almost degenerate edge states is populated in the ground state configuration, the upper state is vacant. As a result, in Fig. 6 a pronounced harmonic yield below the band gap due to incomplete destructive interference is observed, as in the pure phase-B result (cf. Fig. 2b in the Letter).

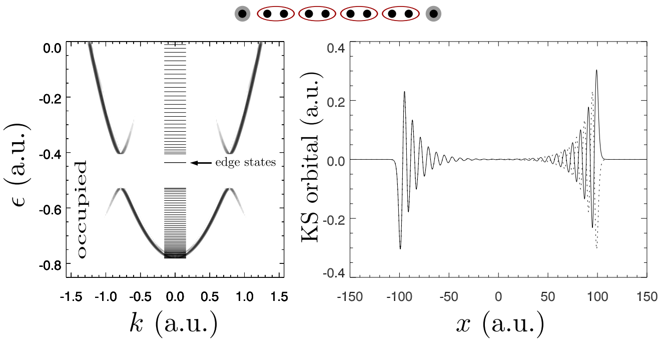


Figure 5. Left: Band structures for the spin-neutral phase B with $N = 100$, $N_\uparrow = N_\downarrow = N/2$, $a = 2$, $\delta = -0.165$ but with impurity ions with smoothing parameter $\varepsilon = 2$ at the left and the right boundary. The edge-state levels are shifted upwards as compared to $\varepsilon = 1$. The edge Right: KS orbitals of the two almost degenerate edge states (lower, occupied, odd orbital $\varphi_{50}(x)$ drawn solid; higher, unoccupied, even orbital $\varphi_{51}(x)$ drawn dashed).

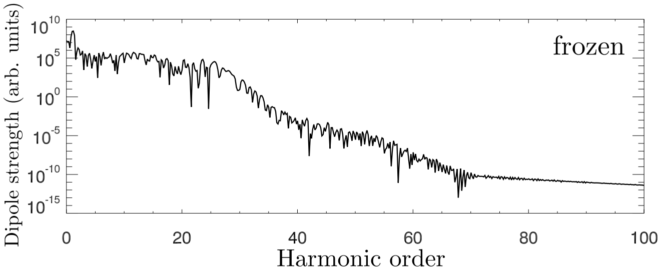


Figure 6. Harmonics emitted by the phase-B chain with $N = 100$ ions, $N_\uparrow = 50$, $N_\downarrow = 50$ and impurity ions at the left and right end. The laser parameters are the same as in the Letter. The result for the frozen KS potential is shown.

## IV. PHASE B WITH AN ADDITIONAL ELECTRON

Our assertion that complete or incomplete destructive interference due to fully or half populated degenerate edge states is the explanation for the absence or presence of sub-band-gap harmonics can be further tested by populating the empty edge state by an additional, “virtual” KS electron. That additional KS electron does not affect the KS potential but its emission is coherently taken into account in the calculation of the harmonics spectrum.

Figure 7 shows that the additional electron *reduces* the harmonic generation in the sub-band-gap region. For comparison, the pure-phase-B spectrum is included. The degree of destructive interference is less than for the phase-A-impurity case in Fig. 4 though because the KS potential (and its level scheme) is not consistent with that additional electron.

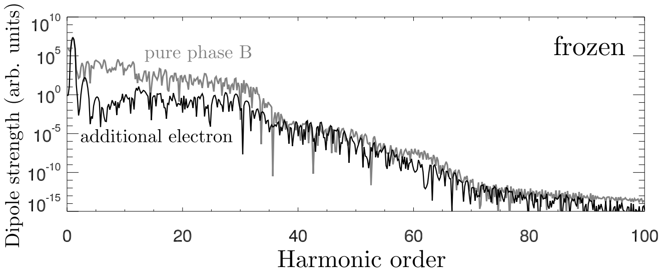


Figure 7. Harmonics emitted by the pure phase-B chain with $N = 100$ ions, $N_\uparrow = 50$, $N_\downarrow = 50$. With an additional, virtual electron populating the second edge state, destructive interference leads to a reduced harmonics emission in the sub-band-gap region (black). For comparison, the original phase-B spectrum is included (gray). The laser parameters are the same as in the Letter. The result for the frozen KS potential is shown (the result for the full KS potential is very similar, as in all the other examples in this work).
